# Supplementary material for: Ultrafast manipulations of nanoscale skyrmioniums
Source: arXiv:2409.00683 source file (2024-09-01)
Supplement: Supplementary file 1 [file Supplementary_Materials.pdf]

# Supplementary Materials for
### "Ultrafast manipulations of nanoscale skyrmioniums"

## S1. Micromagnetic simulations

We used the open-source software Mumax3 for the micromagnetic simulations. With the assistance of our large-scale GPU-based computational servers, Mumax3 is able to conduct computationally intensive and high-throughput simulations involving micromagnetic processes. To obtain the phase diagrams for the magnetic structure of a single-layer magnet, we set the cell size of the simulations to 1 nm × 1 nm × 0.4 nm, and the cell size is smaller than the exchange length for the whole simulations. The grid size in the *xy* direction to 512 × 512, and the periodic boundary conditions are (5, 5, 0). All the simulations are performed in zero magnetic fields, the saturation magnetization $M_s$ = 914 kA/m, the Gilbert damping factor $\alpha$ = 0.1, and the temperature $T$ = 4.2 K is fixed in the whole simulations, and the initial state is a random magnetization state. The effects of the magnetic parameters on the spin structures are investigated by controlling one of the exchange stiffness (interaction) A, the DMI value D, and t perpendicular magnetic anisotropy (PMA) constant $K_u$ to be constant. For example, $K_u$ =6 MJ/m$^3$, $D$=9.1 mJ/m$^2$, and $A$=11.2 pJ/m in Fig. 1 (a), (b), and (c) respectively. The corresponding values of the magnetic parameters are taken concerning our previous work [1].

To obtain skyrmions and skyrmioniums in nanodiscs, the magnetic parameters we used here are as follows: the exchange interaction constant $A$=11.2 pJ/m, $K_u$=5.9 MJ/m$^3$, $D$=9 mJ/m$^2$, but Gilbert damping factor $\alpha$ is set to 0.012 here, the number of grids is 160 × 160 × 1, the cell mesh size is 0.5 nm × 0.5 nm × 0.5 nm, and the thickness of the disk is 0.4 nm. There are no natural materials with such magnetic parameters, but we hope that, in the future, similar artificial magnetic materials or heterostructures can be prepared. We hope that the theoretical study will establish a theoretical framework for the experimental study, thereby reducing experimental time and resources. The initial magnetization states are set to vortex states for relaxation. The period of spiral states is about $L_0 = 2\pi \frac{2A}{D} = 15.6$ nm in nanostructures [2]. The effect of external fields, such as the magnetic fields and spin-currents can be included in the LLG equation. The spin transfer torque (STT) of the Slonczewski model induced by spin-polarized currents can be included in LLG equations. In the study of spin-polarized current-driven skyrmioniums, we choose the Slonczewski parameter $\Lambda$ = 1 in the spacer layer, the

current polarizability $P = 0.5$, $\epsilon' = 0$, and the spin direction of the pinned layer is (0, -1, 0). An initial state of Néel-type skyrmioniums is set and relaxed to a steady state [3].

## S2. The magnetization configurations

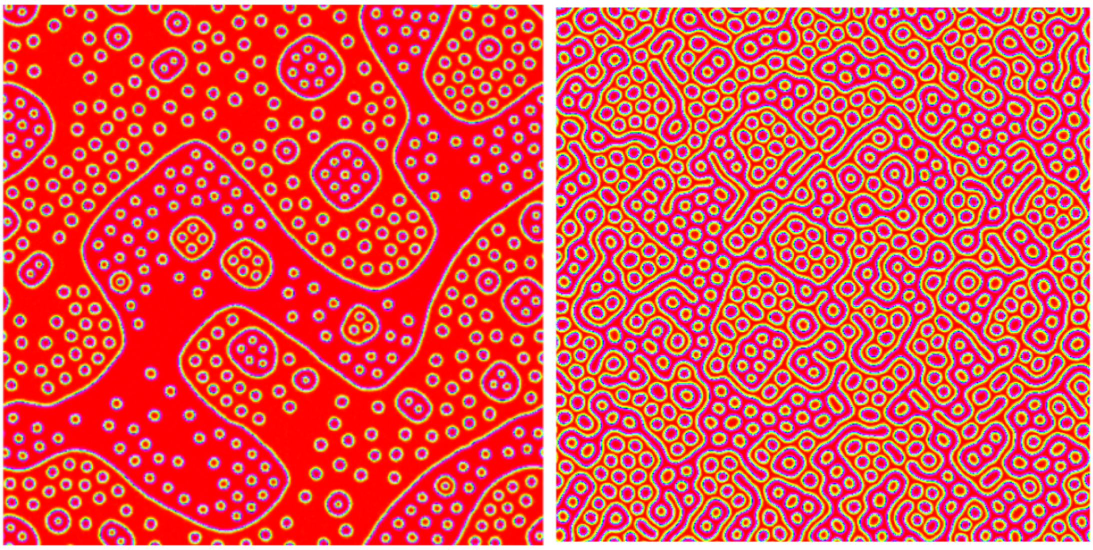

Fig. S1 The magnetization $m_z$ configurations
in phases III (left) and IV (right) for 512 × 512 nm.

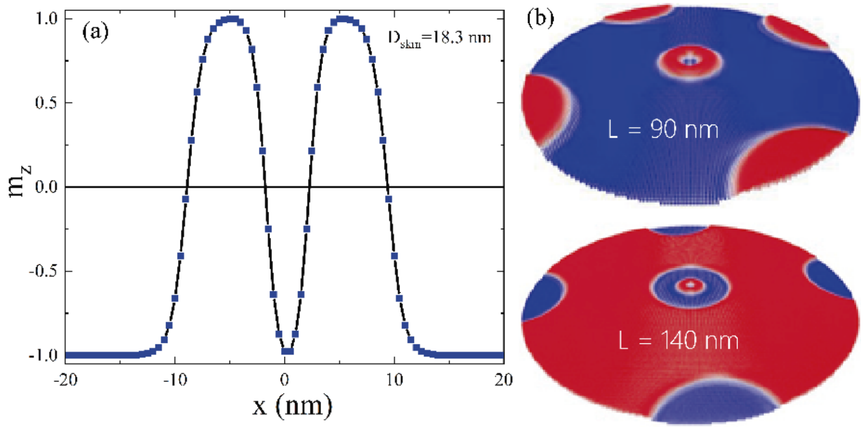


Fig. S2 (a) The magnetization profile $m_z$ at the center of the skyrmionium in a nanodisk with a diameter L=80 nm. (b) The skyrmionium (upper) and $3\pi$-skyrmion (lower) for L=90 and L=140 nm respectively.

## S3. Dynamics of skyrmioniums

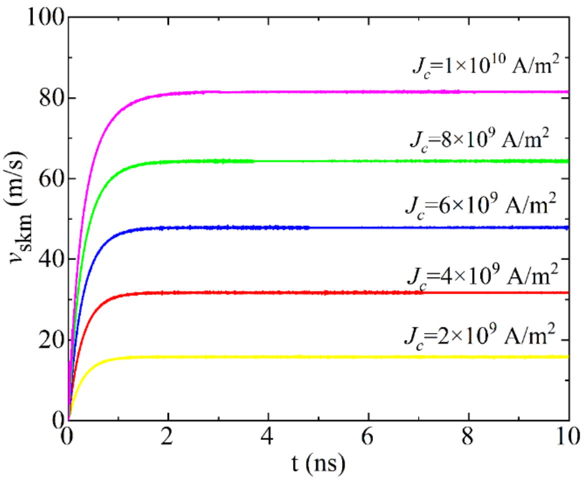


Fig. S3 Temporal evolution of velocities of a skyrmionium for different driving spin-current densities $J_c$.

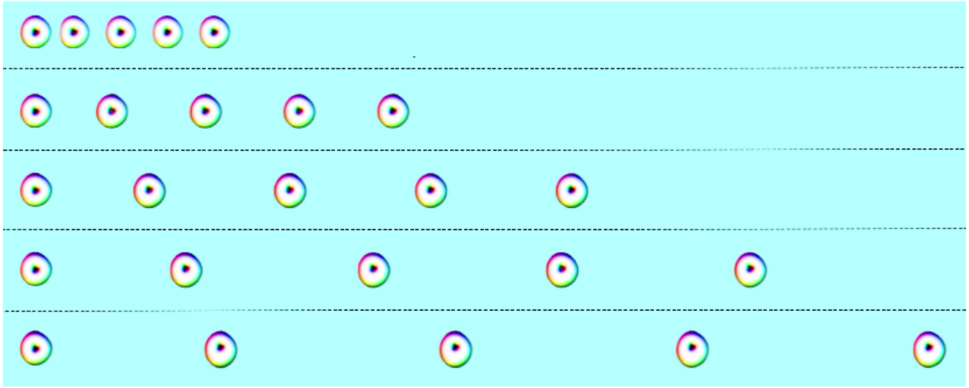

Fig. S4 Snapshots of the skyrmioniums in FM nanoribbons at different driving spin-current densities $J_c$, shown in Fig. S3.

## S4. Temporal evolution of magnetic energy

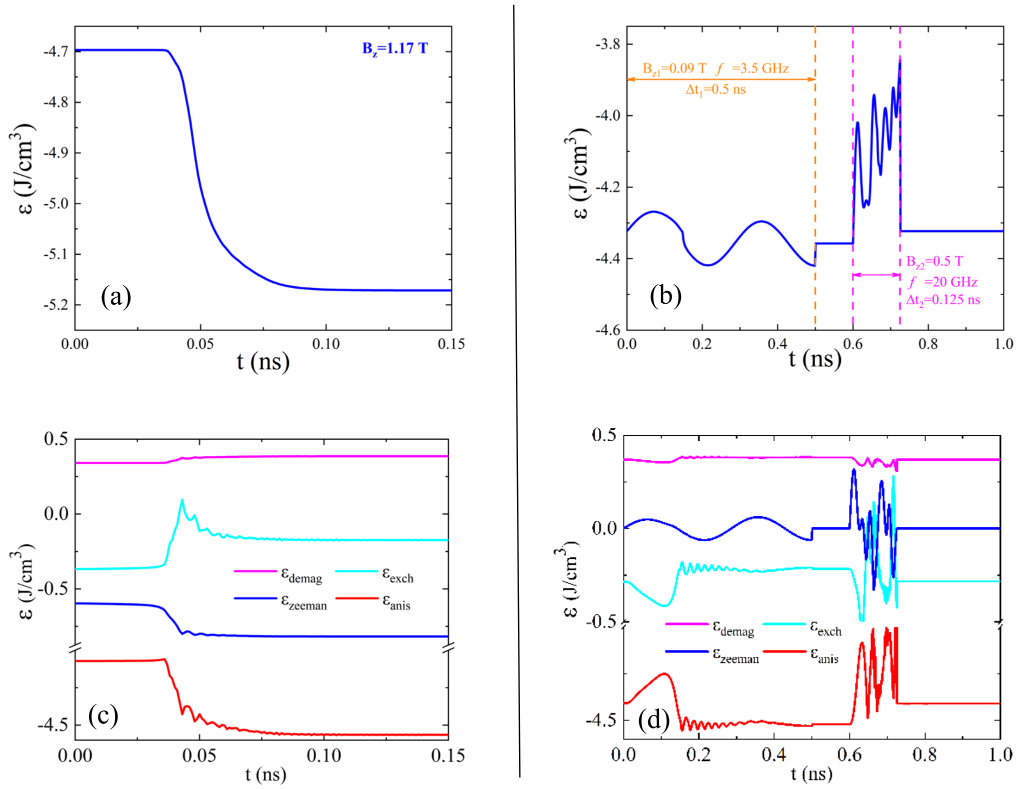


Fig. S5 Temporal evolution of total magnetic energy densities ε at (a) steady magnetic fields, (b) AC magnetic fields. (c) and (d) Temporal evolution of the different involved energy densities ε, respectively for (a) and (b).

## S5. The magnetic force microscopy images and the spin textures

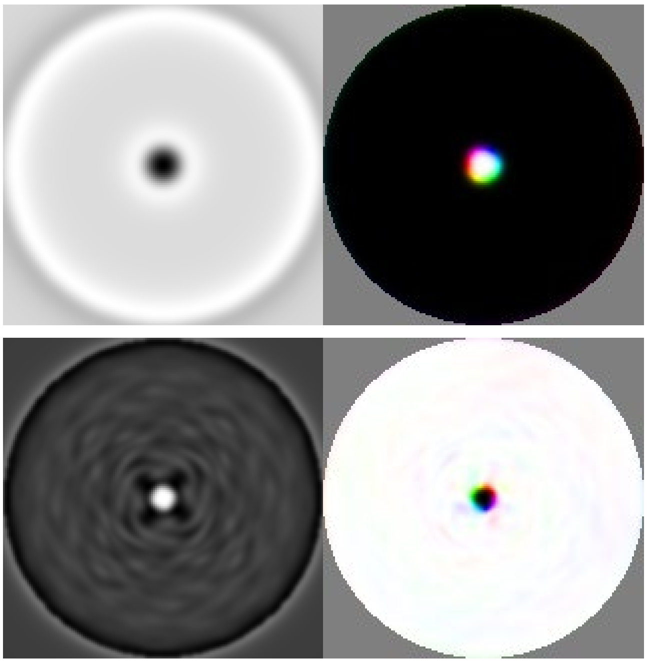

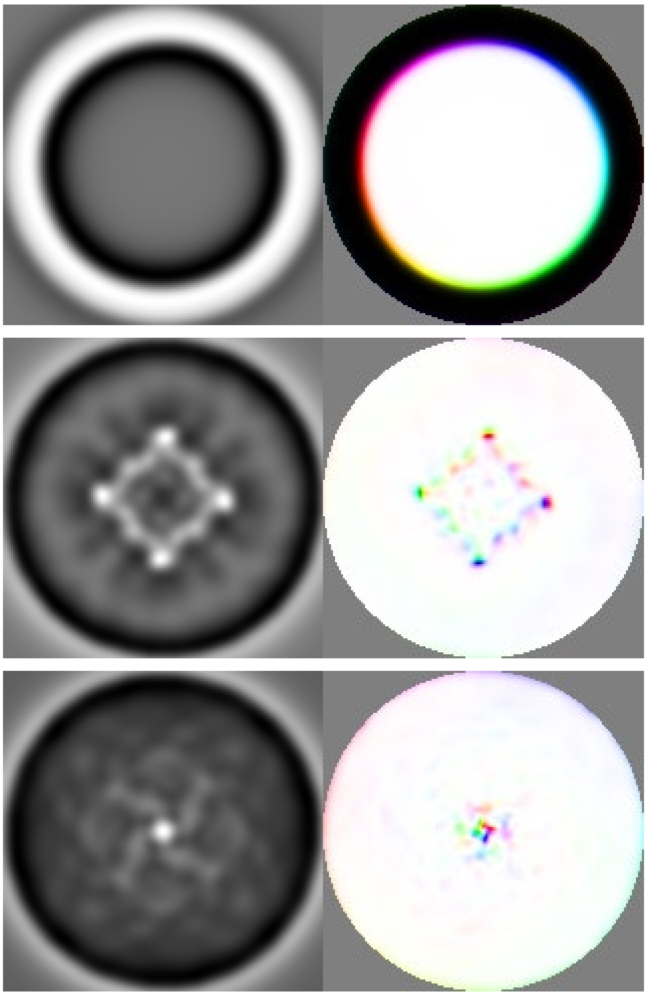

Fig. S6 The stimulated magnetic force microscopy images (left) and the corresponding spin textures (right) under alternating magnetic fields.

**Reference**

[1]. H. M. Dong, P. P. Fu, Y. F. Duan and K. Chang, Nanoscale 15, 15643 (2023).

[2]. J. J. Joos, P. Bassirian, P. Gypens, J. Mulkers, K. Litzius, B. Van Waeyenberge, and J. Leliaert, J. Appl. Phys. 134, 171101 (2023)
